# Supplementary material for: Towards Zero Memory Footprint Spiking Neural Network Training
Source: arXiv:2308.08649 source file (2023-08-16)
Supplement: Supplementary file 1 [file Appendix.tex]

\section{Appendix}
% Optionally include extra information (complete proofs, additional experiments and plots) in the appendix.
% This section will often be part of the supplemental material.
\subsection{Gradient Derivation Process}
This section describes the derivation of 
% Eq.\ref{eq:Inverse_dY/dx_1} and Eq.\ref{eq:Inverse_dY/dx_2}
Eq.13 and Eq.14:

Since we split the input value $X$ into two parts, we need to calculate the gradient of the output value for these two parts separately:

For $X_1$:
\begin{equation}
\frac{\partial \mathbf{Y} }{\partial \mathbf{X_1}}= \frac{\partial \mathbf{Y_1} }{\partial \mathbf{X_1}} + \frac{\partial \mathbf{Y_2}}{\partial \mathbf{X_1}}
\end{equation}

% Based on Eq.\ref{eq:forward Y0} and Eq.\ref{eq:forward Y1}:
Based on Eq.4 and Eq.7:
\begin{equation}
\frac{\partial \mathbf{Y} }{\partial \mathbf{X_1}}= \frac{\partial \left(H\left(M_1 - V_{th}\right) + \beta \cdot X_2^t\right)}{\partial M_1} \odot \frac{\partial M_1^{t}}{\partial {X_1}} +\frac{\partial \left(H\left(M_2 - V_{th}\right) + \beta \cdot X_1^t\right)}{\partial M_2} \odot \frac{\partial M_2}{\partial {X_1}}
\end{equation}

% Based on Eq.\ref{eq:forward M0}, Eq.\ref{eq:forward Y0} and Eq.\ref{eq:forward M1}:
Based on Eq.3, Eq.4 and Eq.6:
\begin{equation}
\frac{\partial \mathbf{Y} }{\partial \mathbf{X_1}}= \frac{\partial H\left(M_1 - V_{th}\right)}{\partial M_1} \odot \frac{1}{\tau} +\frac{\partial H\left(M_2 - V_{th}\right)}{\partial M_2} \odot \frac{1}{\tau} \odot \frac{\partial H\left(M_1 - V_{th}\right)}{\partial M_1} \odot \frac{1}{\tau} + \beta
\end{equation}

The derivative function of the leapfrog equation is defined in pytorch as follows:
\begin{equation}
\frac{\partial H\left(M\right)}{\partial M} = \frac{\theta}{2} \cdot \frac{1}{1+\left(\frac{\pi}{2} \cdot \theta \cdot M \right)^2}
\end{equation}

Then, we can get 
% Eq.\ref{eq:Inverse_dY/dx_1}, and for Eq.\ref{eq:Inverse_dY/dx_2},
Eq.13, and for Eq.14, 
the derivation method is the same.

% For $X_2$:
% \begin{equation}
% \frac{\partial \mathbf{Y} }{\partial \mathbf{X_2}}= \frac{\partial \mathbf{Y_1} }{\partial \mathbf{X_2}} + \frac{\partial \mathbf{Y_2}}{\partial \mathbf{X_2}}
% \end{equation}

% % Based on Eq.\ref{eq:forward Y0} and Eq.\ref{eq:forward Y1}:
% Based on Eq.4 and Eq.7:
% \begin{equation}
% \frac{\partial \mathbf{Y} }{\partial \mathbf{X_2}}= \frac{\partial \left(H\left(M_1 - V_{th}\right) + \beta \cdot X_2^t\right)}{\partial X_2} +\frac{\partial \left(H\left(M_2 - V_{th}\right) + \beta \cdot X_1^t\right)}{\partial M_2} \odot \frac{\partial M_2}{\partial {X_2}}
% \end{equation}

% % Based on Eq.\ref{eq:forward M0}, Eq.\ref{eq:forward Y0} and Eq.\ref{eq:forward M1}:
% Based on Eq.3, Eq.4 and Eq.6:
% \begin{equation}
% \frac{\partial \mathbf{Y} }{\partial \mathbf{X_2}}= \frac{\partial H\left(M_1 - V_{th}\right)}{\partial M_1} \odot \frac{1}{\tau} +\frac{\partial H\left(M_2 - V_{th}\right)}{\partial M_2} \odot \frac{1}{\tau} \odot \frac{\partial H\left(M_1 - V_{th}\right)}{\partial M_1} \odot \frac{1}{\tau} + \beta
% \end{equation}

\subsection{FLOPS Analysis}

For each layer $n$, consider the Input tensor $X^n$ contains $k_n$ elements, for the forward process, 
% Eq.\ref{eq:forward M0}
Eq.3
contains three calculation steps, 
% Eq.\ref{eq:forward Y0}
Eq.4
contains three calculation steps, 
% Eq.\ref{eq:forward V0}
Eq.5
contains six calculation steps. 
% Eq.\ref{eq:forward M1},Eq.\ref{eq:forward V1}, Eq.\ref{eq:forward Y1}
Eq.6,Eq.7,Eq.8
are perfectly symmetrical with the first three steps. Due to we first divided the matrix into segments, so the total FLOPS for the Forward process of each layer is $12 \times k_n$.

For the inverse process, gradient calculation based on the forward computation graph and gradient calculation based on the inverse computation graph, the FLOPS calculation is similar to the forward process. They need $17 \times k_n$, $15.5 \times k_n$, and $8.5 \times k_n$ FLOPS separately. 

If the intermediate activation values are retained 
% (shown in Figure.\ref{fig:inverse gradient}(a))
(shown in Figure.3(a))
, the FLOPS required for the backpropagation process is $15.5 \times k_n$ for each layer. For the previous reversible layer architecture 
% (shown in Figure.\ref{fig:inverse gradient}(b))
(shown in Figure.3(b))
, the FLOPS required for the backpropagation process is $44.5 \times k_n$ for each layer. For our reversible layer architecture 
% (shown in Figure.\ref{fig:inverse gradient}(c))
(shown in Figure.3(c))
, the FLOPS required for the backpropagation process is $25.5 \times k_n$ for each layer. This analysis also coincides with our experimental results.

\subsection{Comparison With The SOTA Methods Experiments Settings}
This section presents the detailed experiment settings for the 
% Section \ref{Comparison with the SOTA Methods}.
Section 5.1. The detailed hyperparameter settings are shown in Table 1.
\begin{table}[htbp]
\label{tab:hyperparameters data}
  \centering
  \caption{The hyperparameter settings for the comparison experiment with the SOTA Methods}
    \begin{tabular}{|c|c|c|c|}
    \hline
    \multicolumn{4}{|c|}{Comparison with the SOTA Methods} \\
    \hline
    dataset & CIFAR10 & CIFAR100 & Tiny-ImageNet \\
    \hline
    batch size & 128   & 128   & 128 \\
    \hline
    learning rate & 0.01  & 0.01  & 0.3 \\
    \hline
    epochs & 400   & 400   & 100 \\
    \hline
    optimizer & SGD   & SGD    & SGD  \\
    \hline
    momentum & 0.9   & 0.9   & 0.9 \\
    \hline
    weight\_decay & 1.00E-05 & 1.00E-05 & 5.00E-04 \\
    \hline
    \end{tabular}%
  \label{tab:addlabel}%
\end{table}%

\subsection{Memory Evaluation Experiment Data}
This section presents the detailed experimental data from 
% Section \ref{Memory Consumption Evaluation}. 
Section 5.2. 
Original memory data comparing reversible SNN nodes and original SNN nodes for VGG configurations is shown in 
% Tabel \ref{tab:Memory VGG1-10} and Table \ref{tab:Memory VGG11-20}. 
Table 2 and Table 3. 
And original memory data comparing reversible SNN nodes and original SNN nodes for ResNet configurations is shown in 
% Table \ref{tab:Memory ResNet11-20}.
Table 4.

\begin{table}[htbp]
\label{tab:Memory VGG1-10}
  \centering
  \caption{Original memory data comparing reversible SNN nodes and original SNN nodes for VGG configurations from timestep 1 to 10.}
  \scalebox{0.7}{
    \begin{tabular}{|c|c|c|c|c|c|c|c|c|c|c|}
    \hline
    \multicolumn{11}{|c|}{\textbf{VGG architectures timesteps 1-10}} \\
    \hline
    \multicolumn{11}{|c|}{\textbf{VGG11}} \bigstrut\\
    \hline
    Timesteps & 1     & 2     & 3     & 4     & 5     & 6     & 7     & 8     & 9     & 10 \\
    \hline
    Origina SNN node memory(MiB) & 298   & 522.5 & 743.5 & 966.5 & 1187.25 & 1410.5 & 1630.25 & 1852.25 & 2075.25 & 2298.5 \\
    \hline
    Reversible SNN node memory(MiB) & 75    & 76    & 79    & 76    & 76.25 & 78.5  & 76    & 78.75 & 77.75 & 79 \\
    \hline
    \multicolumn{11}{|c|}{\textbf{VGG13}} \\
    \hline
    Timesteps & 1     & 2     & 3     & 4     & 5     & 6     & 7     & 8     & 9     & 10 \\
    \hline
    Origina SNN node memory(MiB) & 491   & 858   & 1220  & 1588.75 & 1952.75 & 2318.5 & 2684.25 & 3049.25 & 3416.375 & 3782.5 \\
    \hline
    Reversible SNN node memory(MiB) & 122   & 121   & 120.5 & 123   & 122.75 & 122   & 124.25 & 121.75 & 123   & 122.5 \\
    \hline
    \multicolumn{11}{|c|}{\textbf{VGG16}} \\
    \hline
    Timesteps & 1     & 2     & 3     & 4     & 5     & 6     & 7     & 8     & 9     & 10 \\
    \hline
    Origina SNN node memory(MiB) & 544   & 950   & 1355  & 1759  & 2166  & 2570  & 2976  & 3378  & 3786  & 4192 \\
    \hline
    Reversible SNN node memory(MiB) & 134   & 132   & 135   & 135.5 & 134.5 & 141   & 140.5 & 140.5 & 138   & 140.75 \\
    \hline
    \multicolumn{11}{|c|}{\textbf{VGG19}} \\
    \hline
    Timesteps & 1     & 2     & 3     & 4     & 5     & 6     & 7     & 8     & 9     & 10 \\
    \hline
    Origina SNN node memory(MiB) & 595.5 & 1042  & 1486  & 1930  & 2374  & 2819.75 & 3265  & 3708  & 4150  & 4595 \\
    \hline
    Reversible SNN node memory(MiB) & 147   & 147   & 148   & 146.25 & 147.5 & 152   & 152.5 & 155   & 155.25 & 157.5 \\
    \hline
    \end{tabular}}%
  \label{tab:Memory VGG1-10}%
\end{table}%

\begin{table}[htbp]
\label{tab:Memory VGG11-20}
  \centering
  \caption{Original memory data comparing reversible SNN nodes and original SNN nodes for VGG configurations from timestep 11 to 20.}
  \scalebox{0.7}{
    \begin{tabular}{|c|c|c|c|c|c|c|c|c|c|c|}
    \hline
    \multicolumn{11}{|c|}{\textbf{VGG architectures timesteps 11-20}} \\
    \hline
    \multicolumn{11}{|c|}{\textbf{VGG11}} \bigstrut\\
    \hline
    Timesteps & 11    & 12    & 13    & 14    & 15    & 16    & 17    & 18    & 19    & 20 \\
    \hline
    Origina SNN node memory(MiB) & 2519.5 & 2740.5 & 2964.5 & 3186.375 & 3407.25 & 3627.875 & 3852  & 4074.25 & 4296  & 4518 \\
    \hline
    Reversible SNN node memory(MiB) & 77    & 77    & 80    & 78.375 & 75.25 & 76.375 & 78    & 77.75 & 78.75 & 77.5 \\
    \hline
    \multicolumn{11}{|c|}{\textbf{VGG13}} \\
    \hline
    Timesteps & 11    & 12    & 13    & 14    & 15    & 16    & 17    & 18    & 19    & 20 \\
    \hline
    Origina SNN node memory(MiB) & 4148  & 4513.25 & 4878.5 & 5246.75 & 5612  & 5977.25 & 6344.375 & 6710.5 & 7076  & 7441 \\
    \hline
    Reversible SNN node memory(MiB) & 121.5 & 121.25 & 123   & 122.75 & 121   & 123.75 & 121.5 & 124   & 123.25 & 122.5 \\
    \hline
    \multicolumn{11}{|c|}{\textbf{VGG16}} \\
    \hline
    Timesteps & 11    & 12    & 13    & 14    & 15    & 16    & 17    & 18    & 19    & 20 \\
    \hline
    Origina SNN node memory(MiB) & 4596.5 & 5001.75 & 5404.75 & 5810.75 & 6213.75 & 6620.5 & 7025  & 7429  & 7832  & 8235 \\
    \hline
    Reversible SNN node memory(MiB) & 139.5 & 138.75 & 140.25 & 140   & 139.5 & 139.5 & 138   & 139   & 137   & 138.5 \\
    \hline
    \multicolumn{11}{|c|}{\textbf{VGG19}} \\
    \hline
    Timesteps & 11    & 12    & 13    & 14    & 15    & 16    & 17    & 18    & 19    & 20 \\
    \hline
    Origina SNN node memory(MiB) & 5039  & 5484  & 5929  & 6373  & 6816  & 7258  & 7701  & 8145.5 & 8588  & 9032 \\
    \hline
    Reversible SNN node memory(MiB) & 155   & 156.25 & 154.75 & 158.5 & 158   & 158.25 & 157.5 & 156   & 152.5 & 154 \\
    \hline
    \end{tabular}}%
  \label{tab:Memory VGG11-20}%
\end{table}%

\begin{table}[htbp]
\label{Memory ResNet1-10}
  \centering
  \caption{Original memory data comparing reversible SNN nodes and original SNN nodes for ResNet configurations from timesteps 1 to 10.}
    \scalebox{0.7}{
    \begin{tabular}{|c|c|c|c|c|c|c|c|c|c|c|}
    \hline
    \multicolumn{11}{|c|}{\textbf{ResNet architectures timesteps 1-10}} \\
    \hline
    \multicolumn{11}{|c|}{\textbf{ResNet19}} \\
    \hline
    Timesteps & 1     & 2     & 3     & 4     & 5     & 6     & 7     & 8     & 9     & 10 \\
    \hline
    Origina SNN node memory(MiB) & 670.4 & 1378 & 1987 & 2597 & 3206 & 3812.4 & 4422 & 5031 & 5638  & 6247 \\
    \hline
    Reversible SNN node memory(MiB) & 192 & 225 & 256 & 288 & 320 & 352 & 384 & 416 & 448 & 480 \\
    \hline
    \multicolumn{11}{|c|}{\textbf{ResNet34}} \\
    \hline
    Timesteps & 1     & 2     & 3     & 4     & 5     & 6     & 7     & 8     & 9     & 10 \\
    \hline
    Origina SNN node memory(MiB) & 972.5 & 1722 & 2475 & 3228 & 3980  & 4733 & 5486 & 6238 & 6990  & 7741 \\
    \hline
    Reversible SNN node memory(MiB) & 242 & 274 & 307 & 341 & 370 & 401 & 433 & 464 & 497 & 531 \\
    \hline
    \multicolumn{11}{|c|}{\textbf{ResNet50}} \\
    \hline
    Timesteps & 1     & 2     & 3     & 4     & 5     & 6     & 7     & 8     & 9     & 10 \\
    \hline
    Origina SNN node memory(MiB) & 2971 & 5221 & 7470 & 9724 & 11978 & 14232 & 16481 & 18731 & 20989 & 23240 \\
    \hline
    Reversible SNN node memory(MiB) & 740 & 774 & 803 & 836 & 873 & 902 & 934 & 965 & 996 & 1031 \\
    \hline
    \multicolumn{11}{|c|}{\textbf{ResNet101}} \\
    \hline
    Timesteps & 1     & 2     & 3     & 4     & 5     & 6     & 7     & 8     & 9     & 10 \\
    \hline
    Origina SNN node memory(MiB) & 4662 & 8140 & 11608 & 15087 & 18558 & 22048 & 25513 & 28993 & 32465 & 35954 \\
    \hline
    Reversible SNN node memory(MiB) & 1151 & 1186 & 1216 & 1248 & 1281 & 1314 & 1347 & 1382 & 1410 & 1440 \\
    \hline
    \end{tabular}}%
  \label{tab:Memory ResNet11-20}%
\end{table}%

\subsection{Training Time Evaluation Experiment Data}
This section presents the detailed experimental data from 
% Section \ref{Training time Evaluation}. 
Section 5.3. 
Backward training time data for three different methods from timesteps 1 to 10 is shown in 
% Table \ref{tab:backward time}, 
Table 5, 
and forward training time data for three different methods is shown in 
% Table \ref{tab:forward time}. 
Table 6. 
We only tested the forward time for timsteps 4, 6 and 8.

\begin{table}[htbp]
\label{tab:backward time}
  \centering
  \caption{Original training \textbf{backward} time data for VGG configurations from timesteps 1 to 10. (a): Origianl SNN node,(b): Reversible SNN node with original reversible backpropagation method, (c): Reversible SNN node with our backpropagation method. The Unit of each number: ms.}
  \scalebox{0.8}{
    \begin{tabular}{|c|c|c|c|c|c|c|c|c|c|c|}
    \hline
    \multicolumn{11}{|c|}{\textbf{VGG11}} \bigstrut\\
    \hline
    Timesteps & 1     & 2     & 3     & 4     & 5     & 6     & 7     & 8     & 9     & 10 \\
    \hline
    (a)   & 12.68 & 18.13 & 31.08 & 39.78 & 49.92 & 59.64 & 71.36 & 74.59 & 87.58 & 100.17 \\
    \hline
    (b)   & 22.31 & 47.19 & 55.44 & 66.85 & 85.05 & 88.63 & 100.97 & 117.14 & 124.27 & 140.68 \\
    \hline
    (c)   & 19.11 & 32.85 & 39.92 & 57.79 & 64.95 & 73.95 & 85.21 & 93.00 & 113.74 & 124.48 \\
    \hline
    \multicolumn{11}{|c|}{\textbf{VGG13}} \\
    \hline
    Timesteps & 1     & 2     & 3     & 4     & 5     & 6     & 7     & 8     & 9     & 10 \\
    \hline
    (a)   & 14.84 & 30.56 & 44.85 & 59.21 & 69.50 & 86.61 & 104.24 & 116.89 & 129.91 & 144.79 \\
    \hline
    (b)   & 32.78 & 55.57 & 80.78 & 98.06 & 120.30 & 142.69 & 164.87 & 184.96 & 206.38 & 225.35 \\
    \hline
    (c)   & 24.97 & 43.72 & 64.67 & 83.66 & 103.13 & 122.18 & 136.46 & 151.40 & 165.39 & 189.51 \\
    \hline
    \multicolumn{11}{|c|}{\textbf{VGG16}} \\
    \hline
    Timesteps & 1     & 2     & 3     & 4     & 5     & 6     & 7     & 8     & 9     & 10 \\
    \hline
    (a)   & 16.49 & 34.30 & 53.25 & 66.46 & 81.57 & 101.78 & 118.29 & 138.28 & 150.98 & 178.04 \\
    \hline
    (b)   & 39.02 & 67.28 & 89.73 & 115.53 & 135.51 & 161.96 & 194.41 & 217.10 & 270.88 & 299.63 \\
    \hline
    (c)   & 28.64 & 55.77 & 71.43 & 98.41 & 117.80 & 132.22 & 157.41 & 176.71 & 204.49 & 241.00 \\
    \hline
    \multicolumn{11}{|c|}{\textbf{VGG19}} \\
    \hline
    Timesteps & 1     & 2     & 3     & 4     & 5     & 6     & 7     & 8     & 9     & 10 \\
    \hline
    (a)   & 20.85 & 37.88 & 60.57 & 83.70 & 98.88 & 119.59 & 142.08 & 159.53 & 181.68 & 202.06 \\
    \hline
    (b)   & 47.00 & 75.84 & 105.98 & 144.35 & 176.03 & 192.37 & 236.23 & 284.01 & 298.23 & 325.66 \\
    \hline
    (c)   & 36.50 & 64.47 & 85.73 & 109.13 & 132.40 & 152.03 & 174.11 & 197.11 & 223.19 & 249.19 \\
    \hline
    \end{tabular}}%
  \label{tab:backward time}%
\end{table}%

\begin{table}[htbp]
\label{tab:forward time}
  \centering
  \caption{Original training \textbf{forward} time data for VGG configurations from timesteps 4 to 8. (a):
Origianl SNN node,(b): Reversible SNN node with original reversible backpropagation method, (c):
Reversible SNN node with our backpropagation method. The Unit of each number: ms.}
    \begin{tabular}{|c|c|c|c|}
    \hline
    \multicolumn{4}{|c|}{\textbf{VGG11}} \\
    \hline
    Timesteps & 4     & 6     & 8 \\
    \hline
    (a)   & 35.91 & 42.14 & 51.63 \\
    \hline
    (b)   & 34.00 & 41.19 & 53.44 \\
    \hline
    (c)   & 34.71 & 44.33 & 47.63 \\
    \hline
    \multicolumn{4}{|c|}{\textbf{VGG13}} \\
    \hline
    Timesteps & 4     & 6     & 8 \\
    \hline
    (a)   & 36.06 & 42.39 & 56.93 \\
    \hline
    (b)   & 37.10 & 44.24 & 56.72 \\
    \hline
    (c)   & 35.16 & 47.55 & 54.71 \\
    \hline
    \multicolumn{4}{|c|}{\textbf{VGG16}} \\
    \hline
    Timesteps & 4     & 6     & 8 \\
    \hline
    (a)   & 39.79 & 57.50 & 72.84 \\
    \hline
    (b)   & 40.84 & 60.11 & 75.66 \\
    \hline
    (c)   & 37.65 & 58.78 & 75.15 \\
    \hline
    \multicolumn{4}{|c|}{\textbf{VGG19}} \\
    \hline
    Timesteps & 4     & 6     & 8 \\
    \hline
    (a)   & 41.83 & 69.32 & 80.33 \\
    \hline
    (b)   & 42.77 & 72.40 & 82.37 \\
    \hline
    (c)   & 39.50 & 67.30 & 80.13 \\
    \hline
    \end{tabular}%
  \label{tab:forward time}%
\end{table}%
